# Supplementary material for: FeatUp: A Model-Agnostic Framework for Features at Any Resolution
Source: arXiv:2403.10516 source file (2024-04-01)
Supplement: Supplementary file 1 [file additional_baselines.tex]

\begin{table}[h]
  \centering
  
    \begin{tabular}{r|cc|cc|cc|c}
    \hline
\multicolumn{1}{l|}{} & 
\multicolumn{2}{c|}{\textbf{\begin{tabular}[c]{@{}c@{}}CAM\\ Faithfulness\end{tabular}}} & 
\multicolumn{2}{c|}{\textbf{\begin{tabular}[c]{@{}c@{}}Object\\ Localization\end{tabular}}} & 
\multicolumn{2}{c|}{\textbf{\begin{tabular}[c]{@{}c@{}}Semantic\\ Segmentation\end{tabular}}} & 
\textbf{\begin{tabular}[c]{@{}c@{}}Depth\\ Estimation\end{tabular}} \\
    % & & & & & & &     \\ % blank row
    \hline
    & A.D.$\downarrow$ & A.I. $\uparrow$ & GT \% $\uparrow$ & Top-1 \% $\uparrow$ & Acc. $\uparrow$ & mIoU $\uparrow$ & SSIMSE $\downarrow$ \\
    \hline
    Low-Res & 16.4 & 4.81 & 16.2 & 13.1 & 0.559 & 0.310 & 86.22 \\
    Bilinear & 13.6 & 5.00 & 16.5 & 13.5 & 0.607 & 0.367 & 78.87\\
    U-Net & 13.8 & 5.17 & 16.2 & 13.2 & 0.601 & 0.334 & 73.73 \\
    Strided & 24.4 & 2.00 & 14.4 & 10.8 & 0.595 & 0.348 & 80.02 \\
    Large Image & 35.9 & 1.04 & 14.2 & 9.91 & 0.597 & 0.355 & 104.2 \\
    \hline
    FastFeatUp & {\ul 11.6} & {\ul 5.39} & {\ul 17.0} & {\ul 13.8} & {\ul 0.610} & {\ul 0.368} & {\ul 68.10} \\
    FeatUp & \textbf{9.47} & \textbf{5.59} & \textbf{17.8} & \textbf{14.2} & \textbf{0.621} & \textbf{0.383} & \textbf{66.12} \\
    \hline
  \end{tabular}
        \vspace{.15in}

  \caption{Comparison of feature upsamplers across a variety of downstream tasks. FeatUp and FastFeatUp consistently outperform baselines, including the learned U-Net and large feature map obtained from a higher-resolution input image.}
  \label{tab:main_results}
      \vspace{-.15in}
\end{table}
